# Supplementary material for: Tikhonov-Fenichel Reductions and their Application to a Novel Modelling Approach for Mutualism
Source: arXiv:2501.12069 ancillary file (2025-09-22)
Supplement: Supplementary file 1 [file tfpvs_and_reductions.pdf]

Tikhonov-Fenichel Reductions and their  
Application to a Novel Modelling Approach  
for Mutualism  
**Supplementary Material**

Johannes Apelt      Volkmar Liebscher

August 27, 2025

**List of TFPVs and Reductions for System (1)**

## TFPV 1

$$\begin{aligned}\pi^* &= (0, 0, 0, 0, 0, 0, 0, \eta) \\ f(x, \tilde{\pi}) &= \begin{pmatrix} -\eta SH \\ -\eta SH \\ \eta SH \end{pmatrix} + \varepsilon \begin{pmatrix} \mu_1 C \left(1 - \frac{H}{K_1}\right) - \delta_1 H \\ \beta_2 S \left(1 - \frac{S}{K_2}\right) - \delta_2 S + \mu_2 C \left(1 - \frac{S}{K_2}\right) \\ \beta_3 C \left(1 - \frac{C}{K_3}\right) - \delta_3 C \end{pmatrix} \\ \mathcal{V}(f^{(0)}) &= \mathcal{V}(S) \cup \mathcal{V}(H)\end{aligned}$$

### Reduction (a)

$$\begin{aligned}\mathcal{M}_0 &= \mathcal{V}(H) = \{ (0, S, C) \mid S, C \in \mathbb{R} \} \\ x_0 &= (0, S', 0), \quad S' > 0 \\ Df^{(0)}(x_0) &= \begin{pmatrix} -\eta S' & 0 & 0 \\ -\eta S' & 0 & 0 \\ \eta S' & 0 & 0 \end{pmatrix} \\ f^{(0)} &= P(x)\psi(x) = \begin{pmatrix} -\eta S \\ -\eta S \\ \eta S \end{pmatrix} \cdot (H)\end{aligned}$$

$$\begin{cases} \dot{S} = \beta_2 S \left(1 - \frac{S}{K_2}\right) - \delta_2 S + \mu_2 C \left(1 - \frac{S}{K_2}\right) - \mu_1 C \\ \dot{C} = \beta_3 C \left(1 - \frac{C}{K_3}\right) - \delta_3 C + \mu_1 C \end{cases}$$

### Reduction (b)

$$\begin{aligned}\mathcal{M}_0 &= \mathcal{V}(S) = \{ (H, 0, C) \mid H, C \in \mathbb{R} \} \\ x_0 &= (H', 0, 0), \quad H' > 0 \\ Df^{(0)}(x_0) &= \begin{pmatrix} 0 & -\eta H' & 0 \\ 0 & -\eta H' & 0 \\ 0 & \eta H' & 0 \end{pmatrix} \\ f^{(0)} &= P(x)\psi(x) = \begin{pmatrix} -\eta H \\ -\eta H \\ \eta H \end{pmatrix} \cdot (S) \\ \begin{cases} \dot{H} = -\delta_1 H + \mu_1 C \left(1 - \frac{H}{K_1}\right) - \mu_2 C \\ \dot{C} = \beta_3 C \left(1 - \frac{C}{K_3}\right) - \delta_3 C + \mu_2 C \end{cases}\end{aligned}$$

## TFPV 2

$$\begin{aligned}
\pi^* &= (0, 0, 0, 0, 0, 0, \mu_2, 0) \\
f(x, \tilde{\pi}) &= \begin{pmatrix} 0 \\ \mu_2 C \left(1 - \frac{S}{K_2}\right) \\ 0 \end{pmatrix} + \varepsilon \begin{pmatrix} -\delta_1 H - \eta SH + \mu_1 C \left(1 - \frac{H}{K_1}\right) \\ \beta_2 S \left(1 - \frac{S}{K_2}\right) - \delta_2 S - \eta SH \\ \beta_3 C \left(1 - \frac{C}{K_3}\right) - \delta_3 C + \eta SH \end{pmatrix} \\
\mathcal{V}(f^{(0)}) &= \mathcal{V}(C) \cup \mathcal{V}(S - K_2) \\
\mathcal{M}_0 &= \{ (H, K_2, C) \mid H, C \in \mathbb{R} \} \\
x_0 &= (0, 0, 0) \\
Df^{(0)}(x_0) &= \begin{pmatrix} 0 & 0 & 0 \\ 0 & -\mu_2 \frac{C}{K_2} & 0 \\ 0 & 0 & 0 \end{pmatrix} \\
f^{(0)} = P(x)\psi(x) &= \begin{pmatrix} 0 \\ \mu_2 C \\ 0 \end{pmatrix} \cdot \left(1 - \frac{S}{K_2}\right) \\
\begin{cases} \dot{H} = -\delta_1 H + \mu_1 C \left(1 - \frac{H}{K_1}\right) - \frac{\eta}{k_2} H \\ \dot{C} = \beta_3 C \left(1 - \frac{C}{K_3}\right) - \delta_3 C + \frac{\eta}{k_2} H \end{cases}
\end{aligned}$$

Note: There is no reduction onto  $\mathcal{V}(C)$ , since there exists no  $x \in \mathcal{V}(C)$  satisfying Theorem 4 (iii).

### TFPV 3

$$\begin{aligned}
\pi^* &= (0, 0, 0, 0, 0, \mu_1, 0, 0) \\
f(x, \tilde{\pi}) &= \begin{pmatrix} \mu_1 C \left(1 - \frac{H}{K_1}\right) \\ 0 \\ 0 \end{pmatrix} + \varepsilon \begin{pmatrix} -\delta_1 H - \eta SH \\ \beta_2 S \left(1 - \frac{S}{K_2}\right) - \delta_2 S - \eta SH + \mu_2 C \left(1 - \frac{S}{K_2}\right) \\ \beta_3 C \left(1 - \frac{C}{K_3}\right) - \delta_3 C + \eta SH \end{pmatrix} \\
\mathcal{V}(f^{(0)}) &= \mathcal{V}(C) \cup \mathcal{V}(H - K_1) \\
\mathcal{M}_0 &= \{ (K_1, S, C) \mid S, C \in \mathbb{R} \} \\
x_0 &= (K_1, S', C'), \quad S', C' > 0 \\
Df^{(0)}(x_0) &= \begin{pmatrix} -\mu_1 \frac{C'}{K_1} & 0 & 0 \\ 0 & 0 & 0 \\ 0 & 0 & 0 \end{pmatrix} \\
f^{(0)} &= P(x)\psi(x) = \begin{pmatrix} \mu_1 C \\ 0 \\ 0 \end{pmatrix} \cdot \left(1 - \frac{H}{K_1}\right) \\
&\begin{cases} \dot{S} = \beta_2 S \left(1 - \frac{S}{K_2}\right) - \delta_2 S + \mu_2 C \left(1 - \frac{S}{K_2}\right) - \frac{\eta}{k_1} S \\ \dot{C} = \beta_3 C \left(1 - \frac{C}{K_3}\right) - \delta_3 C + \frac{\eta}{K_1} S \end{cases}
\end{aligned}$$

Note: There is no reduction onto  $\mathcal{V}(C)$ , since there exists no  $x \in \mathcal{V}(C)$  satisfying Theorem 4 (iii).

## TFPV 4

$$\begin{aligned}
\pi^* &= (0, 0, 0, 0, \delta_3, 0, 0, 0) \\
f(x, \tilde{\pi}) &= \begin{pmatrix} 0 \\ 0 \\ -\delta_3 C \end{pmatrix} + \varepsilon \begin{pmatrix} -\delta_1 H - \eta SH + \mu_1 C \left(1 - \frac{H}{K_1}\right) \\ \beta_2 S \left(1 - \frac{S}{K_2}\right) - \delta_2 S - \eta SH + \mu_2 C \left(1 - \frac{S}{K_2}\right) \\ \beta_3 C \left(1 - \frac{C}{K_3}\right) + \eta SH \end{pmatrix} \\
\mathcal{V}(f^{(0)}) &= \mathcal{V}(C) \\
\mathcal{M}_0 &= \{ (H, S, 0) \mid H, S \in \mathbb{R} \} \\
x_0 &= (0, 0, 0) \\
Df^{(0)}(x_0) &= \begin{pmatrix} 0 & 0 & 0 \\ 0 & 0 & 0 \\ 0 & 0 & -\delta_3 \end{pmatrix} \\
f^{(0)} &= P(x)\psi(x) = \begin{pmatrix} 0 \\ 0 \\ -\delta_3 \end{pmatrix} \cdot (C)
\end{aligned}$$

$$\begin{cases} \dot{H} = -\eta SH - \delta_1 H \\ \dot{S} = -\eta SH + \beta_2 S \left(1 - \frac{S}{K_2}\right) - \delta_2 S \end{cases}$$

## TFPV 5

$$\begin{aligned}
\pi^* &= (0, 0, 0, 0, \delta_3, 0, \mu_2, 0) \\
f(x, \tilde{\pi}) &= \begin{pmatrix} 0 \\ -\mu_2 C \left(1 - \frac{S}{K_2}\right) \\ -\delta_3 C \end{pmatrix} + \varepsilon \begin{pmatrix} -\delta_1 H - \eta SH + \mu_1 C \left(1 - \frac{H}{K_1}\right) \\ \beta_2 S \left(1 - \frac{S}{K_2}\right) - \delta_2 S - \eta SH \\ \beta_3 C \left(1 - \frac{C}{K_3}\right) + \eta SH \end{pmatrix} \\
\mathcal{V}(f^{(0)}) &= \mathcal{V}(C) \\
\mathcal{M}_0 &= \{ (H, S, 0) \mid H, S \in \mathbb{R} \} \\
x_0 &= (0, 0, 0) \\
Df^{(0)}(x_0) &= \begin{pmatrix} 0 & 0 & 0 \\ 0 & 0 & \mu_2 \\ 0 & 0 & -\delta_3 \end{pmatrix} \\
f^{(0)} = P(x)\psi(x) &= \begin{pmatrix} 0 \\ \mu_2 \left(1 - \frac{S}{K_2}\right) \\ -\delta_3 \end{pmatrix} \cdot (C) \\
\begin{cases} \dot{H} = -\eta SH - \delta_1 H \\ \dot{S} = -\eta SH + \beta_2 S \left(1 - \frac{S}{K_2}\right) - \delta_2 S + \frac{\mu_2}{\delta_3} \eta SH \left(1 - \frac{S}{K_2}\right) \end{cases}
\end{aligned}$$

## TFPV 6

$$\begin{aligned}
\pi^* &= (0, 0, 0, 0, \delta_3, \mu_1, 0, 0) \\
f(x, \tilde{\pi}) &= \begin{pmatrix} \mu_1 C \left(1 - \frac{H}{K_1}\right) \\ 0 \\ -\delta_3 C \end{pmatrix} + \varepsilon \begin{pmatrix} -\eta SH - \delta_1 H \\ \beta_2 S \left(1 - \frac{S}{K_2}\right) - \delta_2 S - \eta SH \\ \beta_3 C \left(1 - \frac{C}{K_3}\right) \eta SH \end{pmatrix} \\
\mathcal{V}(f^{(0)}) &= \mathcal{V}(C) \\
\mathcal{M}_0 &= \{ (H, S, 0) \mid H, S \in \mathbb{R} \} \\
x_0 &= (0, 0, 0) \\
Df^{(0)}(x_0) &= \begin{pmatrix} 0 & 0 & \mu_1 \\ 0 & 0 & 0 \\ 0 & 0 & -\delta_3 \end{pmatrix} \\
f^{(0)} = P(x)\psi(x) &= \begin{pmatrix} \mu_1 \left(1 - \frac{H}{K_1}\right) \\ 0 \\ -\delta_3 \end{pmatrix} \cdot (C)
\end{aligned}$$

$$\begin{cases} \dot{H} = -\delta_1 H + \eta \frac{\mu_1 - \delta_3}{\delta_3} \left(1 - \frac{\mu_1}{\mu_1 - \delta_3} \frac{H}{K_1}\right) SH \\ \dot{S} = \beta_2 S \left(1 - \frac{S}{K_2}\right) - \delta_2 S - \eta SH \end{cases}$$

## TFPV 7

$$\begin{aligned}
\pi^* &= (0, 0, 0, 0, \delta_3, \mu_1, \mu_2, 0) \\
f(x, \tilde{\pi}) &= \begin{pmatrix} \mu_1 C \left(1 - \frac{H}{K_1}\right) \\ \mu_2 C \left(1 - \frac{S}{K_2}\right) \\ -\delta_3 C \end{pmatrix} + \varepsilon \begin{pmatrix} -\delta_1 H - \eta SH \\ \beta_2 S \left(1 - \frac{S}{K_2}\right) - \delta_2 S - \eta SH \\ \beta_3 C \left(1 - \frac{C}{K_3}\right) + \eta SH \end{pmatrix} \\
\mathcal{V}(f^{(0)}) &= \mathcal{V}(C) \\
\mathcal{M}_0 &= \{ (H, S, 0) \mid H, S \in \mathbb{R} \} \\
x_0 &= (0, 0, 0) \\
Df^{(0)}(x_0) &= \begin{pmatrix} 0 & 0 & \mu_1 \\ 0 & 0 & \mu_2 \\ 0 & 0 & -\delta_3 \end{pmatrix} \\
f^{(0)} &= P(x)\psi(x) = \begin{pmatrix} \mu_1 \left(1 - \frac{H}{K_1}\right) \\ \mu_2 \left(1 - \frac{S}{K_2}\right) \\ -\delta_3 \end{pmatrix} \cdot (C) \\
\begin{cases} \dot{H} = -\delta_1 H + \eta \frac{\mu_1 - \delta_3}{\delta_3} SH \left(1 - \frac{\mu_1}{\mu_1 - \delta_3} \frac{H}{K_1}\right) \\ \dot{S} = \beta_2 S \left(1 - \frac{S}{K_2}\right) - \delta_2 S + \eta \frac{\mu_2 - \delta_3}{\delta_3} SH \left(1 - \frac{\mu_2}{\mu_2 - \delta_3} \frac{S}{K_2}\right) \end{cases}
\end{aligned}$$

## TFPV 8

$$\pi^* = (0, 0, 0, \delta_2, 0, 0, 0, 0)$$

$$f(x, \tilde{\pi}) = \begin{pmatrix} 0 \\ -\delta_2 S \\ 0 \end{pmatrix} + \varepsilon \begin{pmatrix} -\delta_1 H - \eta SH + \mu_1 C \left(1 - \frac{H}{K_1}\right) \\ \beta_2 S \left(1 - \frac{S}{K_2}\right) - \eta SH + \mu_2 C \left(1 - \frac{S}{K_2}\right) \\ \beta_3 C \left(1 - \frac{C}{K_3}\right) - \delta_3 C + \eta SH \end{pmatrix}$$

$$\mathcal{V}(f^{(0)}) = \mathcal{V}(S)$$

$$\mathcal{M}_0 = \{ (H, 0, C) \mid H, C \in \mathbb{R} \}$$

$$x_0 = (0, 0, 0)$$

$$Df^{(0)}(x_0) = \begin{pmatrix} 0 & 0 & 0 \\ 0 & -\delta_2 & 0 \\ 0 & 0 & 0 \end{pmatrix}$$

$$f^{(0)} = P(x)\psi(x) = \begin{pmatrix} 0 \\ -\delta_2 \\ 0 \end{pmatrix} \cdot (S)$$

$$\begin{cases} \dot{H} = \mu_1 C \left(1 - \frac{H}{K_1}\right) - \delta_1 H \\ \dot{C} = \beta_3 C \left(1 - \frac{C}{K_3}\right) - \delta_3 C \end{cases}$$

## TFPV 9

$$\pi^* = (0, 0, 0, \delta_2, 0, 0, 0, \eta)$$

$$f(x, \tilde{\pi}) = \begin{pmatrix} -\eta SH \\ -\eta SH \\ \eta SH \end{pmatrix} + \varepsilon \begin{pmatrix} -\delta_1 H + \mu_1 C \left(1 - \frac{H}{K_1}\right) \\ \beta_2 S \left(1 - \frac{S}{K_2}\right) - \delta_2 S + \mu_2 C \left(1 - \frac{S}{K_2}\right) \\ \beta_3 C \left(1 - \frac{C}{K_3}\right) - \delta_3 C \end{pmatrix}$$

$$\mathcal{V}(f^{(0)}) = \mathcal{V}(S)$$

$$\mathcal{M}_0 = \{ (H, 0, C) \mid H, C \in \mathbb{R} \}$$

$$x_0 = (0, 0, 0)$$

$$Df^{(0)}(x_0) = \begin{pmatrix} 0 & 0 & 0 \\ 0 & -\delta_2 & 0 \\ 0 & 0 & 0 \end{pmatrix}$$

$$f^{(0)} = P(x)\psi(x) = \begin{pmatrix} -\eta H \\ -\eta H - \delta_2 \\ \eta H \end{pmatrix} \cdot (S)$$

$$\begin{cases} \dot{H} = \mu_1 C \left(1 - \frac{H}{K_1}\right) - \delta_1 H - \mu_2 C \frac{\eta H}{\eta H + \delta_2} \\ \dot{C} = \beta_3 C \left(1 - \frac{C}{K_3}\right) - \delta_3 C + \mu_2 C \frac{\eta H}{\eta H + \delta_2} \end{cases}$$

## TFPV 10

$$\begin{aligned}
\pi^* &= (0, 0, 0, \delta_2, 0, 0, \mu_2, 0) \\
f(x, \pi) &= \begin{pmatrix} 0 \\ \mu_2 C \left(1 - \frac{S}{K_2}\right) - \delta_2 S \\ 0 \end{pmatrix} + \varepsilon \begin{pmatrix} -\delta_1 H - \eta SH + \mu_1 C \left(1 - \frac{H}{K_1}\right) \\ \beta_2 S \left(1 - \frac{S}{K_2}\right) - \eta SH \\ \beta_3 C \left(1 - \frac{C}{K_3}\right) - \delta_3 C + \eta SH \end{pmatrix} \\
\mathcal{V}(f^{(0)}) &= \mathcal{V} \left( \mu_2 C \left(1 - \frac{S}{K_2}\right) - \delta_2 S \right) \\
\mathcal{M}_0 &= \left\{ \left( H, S, \frac{\delta_2 S}{\mu_2 \left(1 - \frac{S}{K_2}\right)} \right) \mid H, S \in \mathbb{R}, S < K_2 \right\} \\
x_0 &= (0, 0, 0) \\
Df^{(0)}(x_0) &= \begin{pmatrix} 0 & 0 & 0 \\ 0 & -\delta_2 & \mu_2 \\ 0 & 0 & 0 \end{pmatrix} \\
f^{(0)} &= P(x)\psi(x) = \begin{pmatrix} 0 \\ 1 \\ 0 \end{pmatrix} \cdot \left( \mu_2 C \left(1 - \frac{S}{K_2}\right) - \delta_2 S \right) \\
\begin{cases} \dot{H} = -\delta_1 H - \eta SH + \mu_1 \left(1 - \frac{H}{K_1}\right) \frac{\delta_2 S}{\mu_2 \left(1 - \frac{S}{K_2}\right)} \\ \dot{S} = (\beta_3 - \delta_3) S \left(1 - \left(\frac{1}{K_2} + \frac{\delta_2 \beta_3}{\mu_2 (\beta_3 - \delta_3) K_3}\right) S\right) + \eta \frac{\mu_2}{\delta_2} \left(1 - \frac{S}{K_2}\right)^2 SH \end{cases}
\end{aligned}$$

## TFPV 11

$$\begin{aligned}
\pi^* &= (0, 0, \delta_1, 0, 0, 0, 0) \\
f(x, \pi) &= \begin{pmatrix} -\delta_1 H \\ 0 \\ 0 \end{pmatrix} + \varepsilon \begin{pmatrix} -\eta SH + \mu_1 C \left(1 - \frac{H}{K_1}\right) \\ \beta_2 S \left(1 - \frac{S}{K_2}\right) - \delta_2 S - \eta SH + \mu_2 C \left(1 - \frac{S}{K_2}\right) \\ \beta_3 C \left(1 - \frac{C}{K_3}\right) - \delta_3 C + \eta SH \end{pmatrix} \\
\mathcal{V}(f^{(0)}) &= \mathcal{V}(H) \\
\mathcal{M}_0 &= \{ (0, S, C) \mid S, C \in \mathbb{R} \} \\
x_0 &= (0, 0, 0) \\
Df^{(0)}(x_0) &= \begin{pmatrix} -\delta_1 & 0 & 0 \\ 0 & 0 & 0 \\ 0 & 0 & 0 \end{pmatrix} \\
f^{(0)} = P(x)\psi(x) &= \begin{pmatrix} -\delta_1 \\ 0 \\ 0 \end{pmatrix} \cdot (H) \\
&\begin{cases} \dot{S} = \beta_2 S \left(1 - \frac{S}{K_2}\right) - \delta_2 S + \mu_2 C \left(1 - \frac{S}{K_2}\right) \\ \dot{C} = \beta_3 C \left(1 - \frac{C}{K_3}\right) - \delta_3 C \end{cases}
\end{aligned}$$

## TFPV 12

$$\begin{aligned}
\pi^* &= (0, 0, \delta_1, 0, 0, 0, 0, \eta) \\
f(x, \pi) &= \begin{pmatrix} -\delta_1 H - \eta S H \\ -\eta S H \\ \eta S H \end{pmatrix} + \varepsilon \begin{pmatrix} \mu_1 C \left(1 - \frac{H}{K_1}\right) \\ \beta_2 S \left(1 - \frac{S}{K_2}\right) - \delta_2 S + \mu_2 C \left(1 - \frac{S}{K_2}\right) \\ \beta_3 C \left(1 - \frac{C}{K_3}\right) - \delta_3 C \end{pmatrix} \\
\mathcal{V}(f^{(0)}) &= \mathcal{V}(H) \\
\mathcal{M}_0 &= \{ (0, S, C) \mid S, C \in \mathbb{R} \} \\
x_0 &= (0, 0, 0) \\
Df^{(0)}(x_0) &= \begin{pmatrix} -\delta_1 & 0 & 0 \\ 0 & 0 & 0 \\ 0 & 0 & 0 \end{pmatrix} \\
f^{(0)} &= P(x)\psi(x) = \begin{pmatrix} -\eta S - \delta_1 \\ -\eta S \\ \eta S \end{pmatrix} \cdot (H) \\
\begin{cases} \dot{S} = \beta_2 S \left(1 - \frac{S}{K_2}\right) - \delta_2 S + \mu_2 C \left(1 - \frac{S}{K_2}\right) - \mu_1 C \frac{\eta S}{\eta S + \delta_1} \\ \dot{C} = \beta_3 C \left(1 - \frac{C}{K_3}\right) - \delta_3 C + \mu_1 C \frac{\eta S}{\eta S + \delta_1} \end{cases}
\end{aligned}$$

### TFPV 13

$$\begin{aligned}
\pi^* &= (0, 0, \delta_1, 0, 0, \mu_1, 0, 0) \\
f(x, \tilde{\pi}) &= \begin{pmatrix} \mu_1 C \left(1 - \frac{H}{K_1}\right) - \delta_1 H \\ 0 \\ 0 \end{pmatrix} + \varepsilon \begin{pmatrix} -\eta SH \\ \beta_2 S \left(1 - \frac{S}{K_2}\right) - \delta_2 S - \eta SH + \mu_2 C \left(1 - \frac{S}{K_2}\right) \\ \beta_3 C \left(1 - \frac{C}{K_3}\right) - \delta_3 C + \eta SH \end{pmatrix} \\
\mathcal{V}(f^{(0)}) &= \mathcal{V} \left( \mu_1 C \left(1 - \frac{H}{K_1}\right) - \delta_1 H \right) \\
\mathcal{M}_0 &= \left\{ \left( H, S, \frac{\delta_1 H}{\mu_1 \left(1 - \frac{H}{K_1}\right)} \right) \mid H, S \in \mathbb{R}, H < K_1 \right\} \\
x_0 &= (0, 0, 0) \\
Df^{(0)}(x_0) &= \begin{pmatrix} -\delta_1 & 0 & \mu_1 \\ 0 & 0 & 0 \\ 0 & 0 & 0 \end{pmatrix} \\
f^{(0)} &= P(x)\psi(x) = \begin{pmatrix} 1 \\ 0 \\ 0 \end{pmatrix} \cdot \left( \mu_1 C \left(1 - \frac{H}{K_1}\right) - \delta_1 H \right) \\
\begin{cases} \dot{H} = (\beta_3 - \delta_3) H \left(1 - \left( \frac{1}{K_1} + \frac{\beta_3 \delta_1}{\mu_1 (\beta_3 - \delta_3) K_3} \right) H \right) + \eta \frac{\mu_1}{\delta_1} \left(1 - \frac{H}{K_1}\right)^2 SH \\ \dot{S} = \beta_2 S \left(1 - \frac{S}{K_2}\right) - \delta_2 S - \eta SH + \mu_2 \left(1 - \frac{S}{K_2}\right) \frac{\delta_1 H}{\mu_1 \left(1 - \frac{H}{K_1}\right)} \end{cases}
\end{aligned}$$

## TFPV 14

$$\begin{aligned}\pi^* &= (0, \beta_3, 0, 0, 0, 0, 0) \\ f(x, \pi) &= \begin{pmatrix} 0 \\ 0 \\ \beta_3 C \left(1 - \frac{C}{K_3}\right) \end{pmatrix} + \varepsilon \begin{pmatrix} -\delta_1 H - \eta SH + \mu_1 C \left(1 - \frac{H}{K_1}\right) \\ \beta_2 S \left(1 - \frac{S}{K_2}\right) - \delta_2 S - \eta SH + \mu_2 C \left(1 - \frac{S}{K_2}\right) \\ -\delta_3 C + \eta SH \end{pmatrix} \\ \mathcal{V}(f^{(0)}) &= \mathcal{V}(C) \cup \mathcal{V}(C - K_3)\end{aligned}$$

### Reduction (a)

$$\begin{aligned}\mathcal{M}_0 &= \mathcal{V}(C) = \{ (H, S, 0) \mid H, S \in \mathbb{R} \} \\ x_0 &= (0, 0, 0) \\ Df^{(0)}(x_0) &= \begin{pmatrix} 0 & 0 & 0 \\ 0 & 0 & 0 \\ 0 & 0 & \beta_3 \end{pmatrix} \\ f^{(0)} &= P(x)\psi(x) = \begin{pmatrix} 0 \\ 0 \\ \beta_3 \left(1 - \frac{C}{K_3}\right) \end{pmatrix} \cdot (C) \\ &\begin{cases} \dot{H} = -\eta SH - \delta_1 H \\ \dot{S} = -\eta SH + \beta_2 S \left(1 - \frac{S}{K_2}\right) - \delta_2 S \end{cases}\end{aligned}$$

### Reduction (b)

$$\begin{aligned}\mathcal{M}_0 &= \mathcal{V}(C - K_3) = \{ (H, S, K_3) \mid H, S \in \mathbb{R} \} \\ x_0 &= (0, 0, K_3) \\ Df^{(0)}(x_0) &= \begin{pmatrix} 0 & 0 & 0 \\ 0 & 0 & 0 \\ 0 & 0 & -\beta_3 \end{pmatrix} \\ f^{(0)} &= P(x)\psi(x) = \begin{pmatrix} 0 \\ 0 \\ \beta_3 \left(1 - \frac{C}{K_3}\right) \end{pmatrix} \cdot (C) \\ &\begin{cases} \dot{H} = -\delta_1 H - \eta SH + \mu_1 K_3 \left(1 - \frac{H}{K_1}\right) \\ \dot{S} = \beta_2 S \left(1 - \frac{S}{K_2}\right) - \delta_2 S - \eta SH + \mu_2 K_3 \left(1 - \frac{S}{K_2}\right) \end{cases}\end{aligned}$$

## TFPV 15

$$\begin{aligned}
\pi^* &= (0, \beta_3, 0, 0, 0, 0, \mu_2, 0) \\
f(x, \tilde{\pi}) &= \begin{pmatrix} 0 \\ \mu_2 C \left(1 - \frac{S}{K_2}\right) \\ \beta_3 C \left(1 - \frac{C}{K_3}\right) \end{pmatrix} + \varepsilon \begin{pmatrix} -\delta_1 H - \eta SH + \mu_1 C \left(1 - \frac{H}{K_1}\right) \\ \beta_2 S \left(1 - \frac{S}{K_2}\right) - \delta_2 S - \eta SH \\ -\delta_3 C + \eta SH \end{pmatrix} \\
\mathcal{V}(f^{(0)}) &= \mathcal{V}(C) \cup \mathcal{V}(C - K_3, S - K_2) \\
\mathcal{M}_0 &= \{ (H, S, 0) \mid H, S \in \mathbb{R} \} \\
x_0 &= (0, 0, 0) \\
Df^{(0)}(x_0) &= \begin{pmatrix} 0 & 0 & 0 \\ 0 & 0 & \mu_2 \\ 0 & 0 & \beta_3 \end{pmatrix} \\
f^{(0)} &= P(x)\psi(x) = \begin{pmatrix} 0 \\ \mu_2 \left(1 - \frac{S}{K_2}\right) \\ \beta_3 \left(1 - \frac{C}{K_3}\right) \end{pmatrix} \cdot (C) \\
\begin{cases} \dot{H} = (-\delta_1) H - \eta SH \\ \dot{S} = \beta_2 S \left(1 - \frac{S}{K_2}\right) - \delta_2 S - \eta SH - \eta \frac{\mu_2}{\beta_3} \left(1 - \frac{S}{K_2}\right) SH \end{cases}
\end{aligned}$$

## TFVP 16

$$\begin{aligned}
\pi^* &= (0, \beta_3, 0, 0, 0, \mu_1, 0, 0) \\
f(x, \tilde{\pi}) &= \begin{pmatrix} \mu_1 C \left(1 - \frac{H}{K_1}\right) \\ 0 \\ \beta_3 C \left(1 - \frac{C}{K_3}\right) \end{pmatrix} + \varepsilon \begin{pmatrix} -\delta_1 H - \eta SH \\ \beta_2 S \left(1 - \frac{S}{K_2}\right) - \delta_2 S - \eta SH + \mu_2 C \left(1 - \frac{S}{K_2}\right) \\ -\delta_3 C + \eta SH \end{pmatrix} \\
\mathcal{V}(f^{(0)}) &= \mathcal{V}(C) \cup \mathcal{V}(C - K_3, H - K_1) \\
\mathcal{M}_0 &= \{ (H, S, 0) \mid H, S \in \mathbb{R} \} \\
x_0 &= (0, 0, 0) \\
Df^{(0)}(x_0) &= \begin{pmatrix} 0 & 0 & \mu_1 \\ 0 & 0 & 0 \\ 0 & 0 & \beta_3 \end{pmatrix} \\
f^{(0)} = P(x)\psi(x) &= \begin{pmatrix} \mu_1 \left(1 - \frac{H}{K_1}\right) \\ 0 \\ \beta_3 \left(1 - \frac{C}{K_3}\right) \end{pmatrix} \cdot (C) \\
&\begin{cases} \dot{H} = -\delta_1 H - \eta \frac{\beta_3 + \mu_1}{\beta_3} SH \left(1 - \frac{\mu_1}{\beta_3 + \mu_1} \frac{H}{K_1}\right) \\ \dot{S} = \beta_2 S \left(1 - \frac{S}{K_2}\right) - \delta_2 S - \eta SH \end{cases}
\end{aligned}$$

## TFPV 17

$$\begin{aligned}
\pi^* &= (0, \beta_3, 0, 0, 0, \mu_1, \mu_2, 0) \\
f(x, \tilde{\pi}) &= \begin{pmatrix} \mu_1 C \left(1 - \frac{H}{K_1}\right) \\ \mu_2 C \left(1 - \frac{S}{K_2}\right) \\ \beta_3 C \left(1 - \frac{C}{K_3}\right) \end{pmatrix} + \varepsilon \begin{pmatrix} -\delta_1 H - \eta SH \\ \beta_2 S \left(1 - \frac{S}{K_2}\right) - \delta_2 S - \eta SH \\ -\delta_3 C + \eta SH \end{pmatrix} \\
\mathcal{V}(f^{(0)}) &= \mathcal{V}(C) \cup \mathcal{V}(C - K_3, S - K_2, H - K_1) \\
\mathcal{M}_0 &= \{ (H, S, 0) \mid H, S \in \mathbb{R} \} \\
x_0 &= (0, 0, 0) \\
Df^{(0)}(x_0) &= \begin{pmatrix} 0 & 0 & \mu_1 \\ 0 & 0 & \mu_2 \\ 0 & 0 & \beta_3 \end{pmatrix} \\
f^{(0)} = P(x)\psi(x) &= \begin{pmatrix} \mu_1 \left(1 - \frac{H}{K_1}\right) \\ \mu_2 \left(1 - \frac{S}{K_2}\right) \\ \beta_3 \left(1 - \frac{C}{K_3}\right) \end{pmatrix} \cdot (C) \\
\begin{cases} \dot{H} = -\delta_1 H - \eta SH - \eta \frac{\mu_1}{\beta_3} \left(1 - \frac{H}{K_1}\right) SH \\ \dot{S} = \beta_2 S \left(1 - \frac{S}{K_2}\right) - \delta_2 S - \eta SH - \eta \frac{\mu_2}{\beta_3} \left(1 - \frac{S}{K_2}\right) SH \end{cases}
\end{aligned}$$

## TFPV 18

$$\begin{aligned}\pi^* &= (0, \beta_3, 0, 0, \delta_3, 0, 0, 0) \\ f(x, \tilde{\pi}) &= \begin{pmatrix} 0 \\ 0 \\ \beta_3 C \left(1 - \frac{C}{K_3}\right) - \delta_3 C \end{pmatrix} + \varepsilon \begin{pmatrix} -\delta_1 H - \eta SH + \mu_1 C \left(1 - \frac{H}{K_1}\right) \\ \beta_2 S \left(1 - \frac{S}{K_2}\right) - \delta_2 S - \eta SH + \mu_2 C \left(1 - \frac{S}{K_2}\right) \\ -\delta_3 C + \eta SH \end{pmatrix} \\ \mathcal{V}(f^{(0)}) &= \mathcal{V}(C) \cup \mathcal{V}\left(\beta_3 \left(1 - \frac{C}{K_3}\right) - \delta_3\right)\end{aligned}$$

### Reduction (a)

$$\begin{aligned}\mathcal{M}_0 &= \{ (H, S, 0) \mid H, S \in \mathbb{R} \} \\ x_0 &= (0, 0, 0) \\ Df^{(0)}(x_0) &= \begin{pmatrix} 0 & 0 & 0 \\ 0 & 0 & 0 \\ 0 & 0 & \beta_3 - \delta_3 \end{pmatrix} \\ f^{(0)} &= P(x)\psi(x) = \begin{pmatrix} 0 \\ 0 \\ \beta_3 \left(1 - \frac{C}{K_3}\right) - \delta_3 \end{pmatrix} \cdot (C) \\ &\begin{cases} \dot{H} = -\eta SH - \delta_1 H \\ \dot{S} = -\eta SH + \beta_2 S \left(1 - \frac{S}{K_2}\right) - \delta_2 S \end{cases}\end{aligned}$$

### Reduction (b)

$$\begin{aligned}\mathcal{M}_0 &= \left\{ \left( H, S, \frac{\beta_3 - \delta_3}{\beta_3} K_3 \right) \mid H, S \in \mathbb{R} \right\} \\ x_0 &= \left( H', S', \frac{\beta_3 - \delta_3}{\beta_3} K_3 \right), \quad H', S' > 0 \\ Df^{(0)}(x_0) &= \begin{pmatrix} 0 & 0 & 0 \\ 0 & 0 & 0 \\ 0 & 0 & -(\beta_3 - \delta_3) \end{pmatrix} \\ f^{(0)} &= P(x)\psi(x) = \begin{pmatrix} 0 \\ 0 \\ C \end{pmatrix} \cdot \left( \beta_3 \left(1 - \frac{C}{K_3}\right) - \delta_3 \right) \\ &\begin{cases} \dot{H} = \frac{\mu_1}{\beta_3} K_3 (\beta_3 - \delta_3) \left(1 - \frac{H}{K_1}\right) - \eta SH - \delta_1 H \\ \dot{S} = \frac{\mu_2}{\beta_3} K_3 (\beta_3 - \delta_3) \left(1 - \frac{S}{K_2}\right) - \eta SH + \beta_2 S \left(1 - \frac{S}{K_2}\right) - \delta_2 S \end{cases}\end{aligned}$$

## TFPV 19

$$\begin{aligned}
\pi^* &= (0, \beta_3, 0, 0, \delta_3, 0, \mu_2, 0) \\
f(x, \pi) &= \begin{pmatrix} 0 \\ \mu_2 C \left(1 - \frac{S}{K_2}\right) \\ \beta_3 C \left(1 - \frac{C}{K_3}\right) - \delta_3 C \end{pmatrix} + \varepsilon \begin{pmatrix} -\delta_1 H - \eta SH + \mu_1 C \left(1 - \frac{H}{K_1}\right) \\ \beta_2 S \left(1 - \frac{S}{K_2}\right) - \delta_2 S - \eta SH \\ \eta SH \end{pmatrix} \\
\mathcal{V}(f^{(0)}) &= \mathcal{V}(C) \cup \mathcal{V} \left( \beta_3 \left(1 - \frac{C}{K_3}\right) - \delta_3, S - K_2 \right) \\
\mathcal{M}_0 &= \{ (H, S, 0) \mid H, S \in \mathbb{R} \} \\
x_0 &= (0, 0, 0) \\
Df^{(0)}(x_0) &= \begin{pmatrix} 0 & 0 & 0 \\ 0 & 0 & \mu_2 \\ 0 & 0 & \beta_3 - \delta_3 \end{pmatrix} \\
f^{(0)} = P(x)\psi(x) &= \begin{pmatrix} 0 \\ \mu_2 \left(1 - \frac{S}{K_2}\right) \\ \beta_3 \left(1 - \frac{C}{K_3}\right) - \delta_3 \end{pmatrix} \cdot (C) \\
\begin{cases} \dot{H} = -\delta_1 H - \eta SH \\ \dot{S} = \beta_2 S \left(1 - \frac{S}{K_2}\right) - \delta_2 S - \eta SH - \eta \frac{\mu_2}{\beta_3 - \delta_3} \left(1 - \frac{S}{K_2}\right) SH \end{cases}
\end{aligned}$$

## TFPV 20

$$\begin{aligned}
\pi^* &= (0, \beta_3, 0, 0, \delta_3, \mu_1, 0, 0) \\
f(x, \pi) &= \begin{pmatrix} \mu_1 C \left(1 - \frac{H}{K_1}\right) \\ 0 \\ \beta_3 C \left(1 - \frac{C}{K_3}\right) - \delta_3 C \end{pmatrix} + \varepsilon \begin{pmatrix} -\delta_1 H - \eta SH + \mu_1 C \left(1 - \frac{H}{K_1}\right) \\ \beta_2 S \left(1 - \frac{S}{K_2}\right) - \delta_2 S - \eta SH + \mu_2 C \left(1 - \frac{S}{K_2}\right) \\ \eta SH \end{pmatrix} \\
\mathcal{V}(f^{(0)}) &= \mathcal{V}(C) \cup \mathcal{V} \left( \beta_3 \left(1 - \frac{C}{K_3}\right) - \delta_3, H - K_1 \right) \\
\mathcal{M}_0 &= \{ (H, S, 0) \mid H, S \in \mathbb{R} \} \\
x_0 &= (0, 0, 0) \\
Df^{(0)}(x_0) &= \begin{pmatrix} 0 & 0 & \mu_1 \\ 0 & 0 & 0 \\ 0 & 0 & \beta_3 - \delta_3 \end{pmatrix} \\
f^{(0)} = P(x)\psi(x) &= \begin{pmatrix} \mu_1 \left(1 - \frac{H}{K_1}\right) \\ 0 \\ \beta_3 \left(1 - \frac{C}{K_3}\right) - \delta_3 \end{pmatrix} \cdot (C) \\
&\begin{cases} \dot{H} = -\delta_1 H - \eta \left(1 + \frac{\mu_1}{\beta_3 - \delta_3} \left(1 - \frac{H}{K_1}\right)\right) SH \\ \dot{S} = \beta_2 S \left(1 - \frac{S}{K_2}\right) - \delta_2 S - \eta SH \end{cases}
\end{aligned}$$

## TFPV 21

$$\begin{aligned}
\pi^* &= (0, \beta_3, 0, 0, \delta_3, \mu_1, \mu_2, 0) \\
f(x, \tilde{\pi}) &= \begin{pmatrix} \mu_1 C \left(1 - \frac{H}{K_1}\right) \\ \mu_2 C \left(1 - \frac{S}{K_2}\right) \\ \beta_3 C \left(1 - \frac{C}{K_3}\right) - \delta_3 C \end{pmatrix} + \varepsilon \begin{pmatrix} -\delta_1 H - \eta SH \\ \beta_2 S \left(1 - \frac{S}{K_2}\right) - \delta_2 S - \eta SH \\ \eta SH \end{pmatrix} \\
\mathcal{V}(f^{(0)}) &= \mathcal{V}(C) \cup \mathcal{V} \left( \beta_3 \left(1 - \frac{C}{K_3}\right) - \delta_3, H - K_1, S - K_2 \right) \\
\mathcal{M}_0 &= \{ (H, S, 0) \mid H, S \in \mathbb{R} \} \\
x_0 &= (0, 0, 0) \\
Df^{(0)}(x_0) &= \begin{pmatrix} 0 & 0 & \mu_1 \\ 0 & 0 & \mu_2 \\ 0 & 0 & \beta_3 - \delta_3 \end{pmatrix} \\
f^{(0)} = P(x)\psi(x) &= \begin{pmatrix} \mu_1 \left(1 - \frac{H}{K_1}\right) \\ \mu_2 \left(1 - \frac{S}{K_2}\right) \\ \beta_3 \left(1 - \frac{C}{K_3}\right) - \delta_3 \end{pmatrix} \cdot (C) \\
\begin{cases} \dot{H} = -\delta_1 H - \eta \left(1 + \frac{\mu_1}{\beta_3 - \delta_3} \left(1 - \frac{H}{K_1}\right)\right) SH \\ \dot{S} = \beta_2 S \left(1 - \frac{S}{K_2}\right) - \delta_2 S - \eta \left(1 + \frac{\mu_2}{\beta_3 - \delta_3} \left(1 - \frac{S}{K_2}\right)\right) SH \end{cases}
\end{aligned}$$

## TFPV 22

$$\begin{aligned}\pi^* &= (\beta_2, 0, 0, 0, 0, 0, 0) \\ f(x, \pi) &= \begin{pmatrix} 0 \\ \beta_2 S \left(1 - \frac{S}{K_2}\right) \\ 0 \end{pmatrix} + \varepsilon \begin{pmatrix} -\delta_1 H - \eta SH + \mu_1 C \left(1 - \frac{H}{K_1}\right) \\ -\delta_2 S - \eta SH + \mu_2 C \left(1 - \frac{S}{K_2}\right) \\ \beta_3 C \left(1 - \frac{C}{K_3}\right) - \delta_3 C + \eta SH \end{pmatrix} \\ \mathcal{V}(f^{(0)}) &= \mathcal{V}(S) \cup \mathcal{V}(S - K_2)\end{aligned}$$

### Reduction (a)

$$\begin{aligned}\mathcal{M}_0 &= \{ (H, 0, C) \mid H, C \in \mathbb{R} \} \\ x_0 &= (0, 0, 0) \\ Df^{(0)}(x_0) &= \begin{pmatrix} 0 & 0 & 0 \\ 0 & \beta_2 & 0 \\ 0 & 0 & 0 \end{pmatrix} \\ f^{(0)} &= P(x)\psi(x) = \begin{pmatrix} 0 \\ \beta_2 \left(1 - \frac{S}{K_2}\right) \\ 0 \end{pmatrix} \cdot (S) \\ &\begin{cases} \dot{H} = \mu_1 C \left(1 - \frac{H}{K_1}\right) - \delta_1 H \\ \dot{C} = \beta_3 C \left(1 - \frac{C}{K_3}\right) - C\delta_3 \end{cases}\end{aligned}$$

### Reduction (b)

$$\begin{aligned}\mathcal{M}_0 &= \{ (H, K_2, C) \mid H, C \in \mathbb{R} \} \\ x_0 &= (0, K_2, 0) \\ Df^{(0)}(x_0) &= \begin{pmatrix} 0 & 0 & 0 \\ 0 & -\beta_2 & 0 \\ 0 & 0 & 0 \end{pmatrix} \\ f^{(0)} &= P(x)\psi(x) = \begin{pmatrix} 0 \\ \beta_2 S \\ 0 \end{pmatrix} \cdot \left( \left(1 - \frac{S}{K_2}\right) \right) \\ &\begin{cases} \dot{H} = -\delta_1 H + \mu_1 C \left(1 - \frac{H}{K_1}\right) - \eta K_2 H \\ \dot{C} = \beta_3 C \left(1 - \frac{C}{K_3}\right) - \delta_3 C + \eta K_2 H \end{cases}\end{aligned}$$

## TFPV 23

$$\begin{aligned}
\pi^* &= (\beta_2, 0, 0, 0, 0, 0, 0, \eta) \\
f(x, \tilde{\pi}) &= \begin{pmatrix} -\eta SH \\ \beta_2 S \left(1 - \frac{S}{K_2}\right) - \eta SH \\ \eta SH \end{pmatrix} + \varepsilon \begin{pmatrix} -\delta_1 H + \mu_1 C \left(1 - \frac{H}{K_1}\right) \\ -\delta_2 S + \mu_2 C \left(1 - \frac{S}{K_2}\right) \\ \beta_3 C \left(1 - \frac{C}{K_3}\right) - \delta_3 C \end{pmatrix} \\
\mathcal{V}(f^{(0)}) &= \mathcal{V}(S) \cup \mathcal{V}(S - K_2, H) \\
\mathcal{M}_0 &= \{ (H, 0, C) \mid H, C \in \mathbb{R} \} \\
x_0 &= (0, 0, 0) \\
Df^{(0)}(x_0) &= \begin{pmatrix} 0 & 0 & 0 \\ 0 & \beta_2 & 0 \\ 0 & 0 & 0 \end{pmatrix} \\
f^{(0)} = P(x)\psi(x) &= \begin{pmatrix} -\eta H \\ \beta_2 \left(1 - \frac{S}{K_2}\right) - \eta H \\ \eta H \end{pmatrix} \cdot (S) \\
\begin{cases} \dot{H} = -\delta_1 H + \mu_1 C \left(1 - \frac{H}{K_1}\right) - \mu_2 C \left(1 + \frac{\beta_2}{\eta H - \beta_2}\right) \\ \dot{C} = \beta_3 C \left(1 - \frac{C}{K_3}\right) - \delta_3 C + \mu_2 C \left(1 + \frac{\beta_2}{\eta H - \beta_2}\right) \end{cases}
\end{aligned}$$

## TFPV 24

$$\begin{aligned}\pi^* &= (\beta_2, 0, 0, 0, 0, 0, \mu_2, 0) \\ f(x, \tilde{\pi}) &= \begin{pmatrix} 0 \\ \beta_2 S \left(1 - \frac{S}{K_2}\right) + \mu_2 C \left(1 - \frac{S}{K_2}\right) \\ 0 \end{pmatrix} + \varepsilon \begin{pmatrix} -\delta_1 H - \eta SH + \mu_1 C \left(1 - \frac{H}{K_1}\right) \\ -\delta_2 S - \eta SH \\ \beta_3 C \left(1 - \frac{C}{K_3}\right) - \delta_3 C + \eta SH \end{pmatrix} \\ \mathcal{V}(f^{(0)}) &= \mathcal{V}(S - K_2) \cup \mathcal{V}(\beta_2 S + \mu_2 C)\end{aligned}$$

### Reduction (a)

$$\begin{aligned}\mathcal{M}_0 &= \mathcal{V}(S - K_2) = \{ (H, K_2, C) \mid H, C \in \mathbb{R} \} \\ x_0 &= (0, K_2, 0) \\ Df^{(0)}(x_0) &= \begin{pmatrix} 0 & 0 & 0 \\ 0 & -\beta_2 & 0 \\ 0 & 0 & 0 \end{pmatrix} \\ f^{(0)} &= P(x)\psi(x) = \begin{pmatrix} 0 \\ \beta_2 S + \mu_2 C \\ 0 \end{pmatrix} \cdot \left(1 - \frac{S}{K_2}\right) \\ \begin{cases} \dot{H} &= -\delta_1 H + \mu_1 C \left(1 - \frac{H}{K_1}\right) - \eta K_2 H \\ \dot{C} &= \beta_3 C \left(1 - \frac{C}{K_3}\right) - \delta_3 C + \eta K_2 H \end{cases}\end{aligned}$$

### Reduction (b)

$$\begin{aligned}\mathcal{M}_0 &= \mathcal{V}(\beta_2 S + \mu_2 C) = \left\{ \left( H, S, \frac{-\beta_2 S}{\mu_2} \right) \mid H, S \in \mathbb{R} \right\} \\ x_0 &= (0, 0, 0) \\ Df^{(0)}(x_0) &= \begin{pmatrix} 0 & 0 & 0 \\ 0 & \beta_2 & \mu_2 \\ 0 & 0 & 0 \end{pmatrix} \\ f^{(0)} &= P(x)\psi(x) = \begin{pmatrix} 0 \\ 1 - \frac{S}{K_2} \\ 0 \end{pmatrix} \cdot (\beta_2 S + \mu_2 C) \\ \begin{cases} \dot{H} &= -\delta_1 H - \eta SH - \beta_2 \frac{\mu_1}{\mu_2} S \left(1 - \frac{H}{K_1}\right) \\ \dot{S} &= \beta_3 S \left(1 + \frac{\beta_2}{\mu_2} \frac{S}{K_3}\right) - \delta_3 S - \eta \frac{\mu_2}{\beta_2} SH \end{cases}\end{aligned}$$

## TFPV 25

$$\begin{aligned}\pi^* &= (\beta_2, 0, 0, \delta_2, 0, 0, 0, 0) \\ f(x, \pi) &= \begin{pmatrix} 0 \\ \beta_2 S \left(1 - \frac{S}{K_2}\right) - \delta_2 S \\ 0 \end{pmatrix} + \varepsilon \begin{pmatrix} -\delta_1 H - \eta SH + \mu_1 C \left(1 - \frac{H}{K_1}\right) \\ -\eta SH + \mu_2 C \left(1 - \frac{S}{K_2}\right) \\ \beta_3 C \left(1 - \frac{C}{K_3}\right) - \delta_3 C + \eta SH \end{pmatrix} \\ \mathcal{V}(f^{(0)}) &= \mathcal{V}(S) \cup \mathcal{V}\left(\beta_2 \left(1 - \frac{S}{K_2}\right) - \delta_2\right)\end{aligned}$$

### Reduction (a)

$$\begin{aligned}\mathcal{M}_0 &= \mathcal{V}(S) = \{ (H, 0, C) \mid H, C \in \mathbb{R} \} \\ x_0 &= (0, 0, 0) \\ Df^{(0)}(x_0) &= \begin{pmatrix} 0 & 0 & 0 \\ 0 & \beta_2 - \delta_2 & 0 \\ 0 & 0 & 0 \end{pmatrix} \\ f^{(0)} &= P(x)\psi(x) = \begin{pmatrix} 0 \\ \beta_2 \left(1 - \frac{S}{K_2}\right) - \delta_2 \end{pmatrix} \cdot (S) \\ &\quad \begin{cases} \dot{H} = \mu_1 C \left(1 - \frac{H}{K_1}\right) - \delta_1 H \\ \dot{C} = \beta_3 C \left(1 - \frac{C}{K_3}\right) - \delta_3 C \end{cases}\end{aligned}$$

### Reduction (b)

$$\begin{aligned}\mathcal{M}_0 &= \mathcal{V}\left(\beta_2 \left(1 - \frac{S}{K_2}\right) - \delta_2\right) = \left\{ \left(H, \frac{\beta_2 - \delta_2}{\beta_2} K_2, C\right) \mid H, C \in \mathbb{R} \right\} \\ x_0 &= \left(0, \frac{\beta_2 - \delta_2}{\beta_2} K_2, 0\right) \\ Df^{(0)}(x_0) &= \begin{pmatrix} 0 & 0 & 0 \\ 0 & -(\beta_2 - \delta_2) & 0 \\ 0 & 0 & 0 \end{pmatrix} \\ f^{(0)} &= P(x)\psi(x) = \begin{pmatrix} 0 \\ S \\ 0 \end{pmatrix} \cdot \left(\left(1 - \frac{S}{K_2}\right) - \delta_2\right) \\ &\quad \begin{cases} \dot{H} = -\delta_1 H + \mu_1 C \left(1 - \frac{H}{K_1}\right) - \eta \frac{\beta_2 - \delta_2}{\beta_2} K_2 H \\ \dot{C} = \beta_3 C \left(1 - \frac{C}{K_3}\right) - \delta_3 C + \eta \frac{\beta_2 - \delta_2}{\beta_2} K_2 H \end{cases}\end{aligned}$$

## TFPV 26

$$\begin{aligned}
\pi^* &= (\beta_2, 0, 0, \delta_2, 0, 0, 0, \eta) \\
f(x, \pi) &= \begin{pmatrix} -\eta SH \\ \beta_2 S \left(1 - \frac{S}{K_2}\right) - \delta_2 S - \eta SH \\ \eta SH \end{pmatrix} + \varepsilon \begin{pmatrix} -\delta_1 H + \mu_1 C \left(1 - \frac{H}{K_1}\right) \\ \mu_2 C \left(1 - \frac{S}{K_2}\right) \\ \beta_3 C \left(1 - \frac{C}{K_3}\right) - \delta_3 C \end{pmatrix} \\
\mathcal{V}(f^{(0)}) &= \mathcal{V}(S) \cup \mathcal{V}\left(\beta_2 \left(1 - \frac{S}{K_2}\right) - \delta_2, H\right) \\
\mathcal{M}_0 &= \{(H, 0, C) \mid H, C \in \mathbb{R}\} \\
x_0 &= (0, 0, 0) \\
Df^{(0)}(x_0) &= \begin{pmatrix} 0 & 0 & 0 \\ 0 & \beta_2 - \delta_2 & 0 \\ 0 & 0 & 0 \end{pmatrix} \\
f^{(0)} = P(x)\psi(x) &= \begin{pmatrix} -\eta H \\ \beta_2 \left(1 - \frac{S}{K_2}\right) - \delta_2 - \eta H \\ \eta H \end{pmatrix} \cdot (S) \\
&\begin{cases} \dot{H} = \mu_1 C \left(1 - \frac{H}{K_1}\right) - \delta_1 H - \mu_2 C \frac{\eta H}{\eta H - (\beta_2 - \delta_2)} \\ \dot{C} = \beta_3 C \left(1 - \frac{C}{K_3}\right) - \delta_3 C + \mu_2 C \frac{\eta H}{\eta H - (\beta_2 - \delta_2)} \end{cases}
\end{aligned}$$

## TFPV 27

$$\begin{aligned}
\pi^* &= (\beta_2, 0, 0, \delta_2, 0, 0, \mu_2, 0) \\
f(x, \bar{\pi}) &= \begin{pmatrix} 0 \\ \beta_2 S \left(1 - \frac{S}{K_2}\right) - \delta_2 S + \mu_2 C \left(1 - \frac{S}{K_2}\right) \\ 0 \end{pmatrix} + \varepsilon \begin{pmatrix} -\delta_1 H - \eta SH + \mu_1 C \left(1 - \frac{H}{K_1}\right) \\ -\eta SH \\ \beta_3 C \left(1 - \frac{C}{K_3}\right) - \delta_3 C + \eta SH \end{pmatrix} \\
\mathcal{V}(f^{(0)}) &= \mathcal{V} \left( \mu_2 C \left(1 - \frac{S}{K_2}\right) + \left( \beta_2 S \left(1 - \frac{S}{K_2}\right) - \delta_2 S \right) S \right) \\
\mathcal{M}_0 &= \left\{ \left( H, S, \frac{\beta_2 S \left(1 - \frac{S}{K_2}\right) - \delta_2 S}{\mu_2 \left(1 - \frac{S}{K_2}\right)} \right) \mid H, S \in \mathbb{R}, S < K_2 \right\} \\
x_0 &= (0, 0, 0) \\
Df^{(0)}(x_0) &= \begin{pmatrix} 0 & 0 & 0 \\ 0 & \beta_2 - \delta_2 & \mu_2 \\ 0 & 0 & 0 \end{pmatrix} \\
f^{(0)} &= P(x)\psi(x) = \begin{pmatrix} 0 \\ 1 \\ 0 \end{pmatrix} \cdot \left( \beta_2 S \left(1 - \frac{S}{K_2}\right) - \delta_2 S + \mu_2 C \left(1 - \frac{S}{K_2}\right) \right) \\
\begin{cases} \dot{H} = -\delta_1 H - \eta SH - \left( \beta_2 S \left(1 - \frac{S}{K_2}\right) - \delta_2 S \right) \frac{\mu_1 \left(1 - \frac{H}{K_1}\right)}{\mu_2 \left(1 - \frac{S}{K_2}\right)} \\ \dot{S} = \frac{(K_2 - S)^2}{\beta_2 (K_2 - S)^2 - \delta_2 K_2^2} S \left( \beta_2 - \frac{\delta_2 K_2}{K_2 - S} \right) \left( \beta_3 \left( 1 + \frac{S}{\mu_2 K_3} \left( \beta_2 - \frac{\delta_2 K_2}{K_2 - S} \right) \right) - \delta_3 \right) \\ \quad + \eta \frac{\mu_2 (K_2 - S)^2}{\delta_2 K_2^2 - \beta_2 (K_2 - S)^2} SH \end{cases}
\end{aligned}$$
